# Supplementary material for: Federated Few-Shot Learning for Mobile NLP
Source: arXiv:2212.05974 source file (2023-08-19)
Supplement: Supplementary file 1 [file sec-appendix-models.tex]

\subsection{Different Foundation Models}\label{sec:appendix-models}
