# Supplementary material for: Federated Few-Shot Learning for Mobile NLP
Source: arXiv:2212.05974 source file (2023-08-19)
Supplement: Supplementary file 2 [file sec-appendix.tex]

\section*{Appendix} \label{sec:appendix}

\subsection{Different Foundation Models}\label{sec:appendix-models}
