# Supplementary material for: Federated Few-Shot Learning for Mobile NLP
Source: arXiv:2212.05974 source file (2023-08-19)
Supplement: Supplementary file 3 [file sec-appendix-models.tex]

\subsection{Different Foundation Models}\label{sec:appendix-models}
This section will show two-fold comparison:

1. Show the gain of few shot fedpet (prompting fine-tuning) versus vanilla fedcls (i.e., head fine-tuning)~\cite{scao2021many}.

2. Show the gap from few shot fedpet versus full dataset fine-tuning.

\input{fig-eval-gain-gap.tex}

End-to-end exps: convergence plots (line plot. X-axis: clock time; Y-axis: testing accuracy).

\textbf{Prompt learning performs better than vanilla fine-tuning.} Uniform few show learning results have been shown in Figure~\ref{fig:eval-gain-gap}.

Experiments todo \mwx{and performance of various models}, shown in Table~\ref{tab:eval-todo}.

\textbf{Performance under various foundation models:}
\mwx{Using 0.1\% data of full-set will enable BERT to perform on par on \texttt{AGNEWS} (0.6, 0.86), \texttt{YAHOO}(0.45, 0.66), \texttt{YELP} (0.27, 0.46), as well. While on \texttt{MNLI}, PET perform on par with CLS (0.48, 0.45). The Full-CLS are almost the same with Roberta-large.}


\input{fig-eval-model.tex}
