# Supplementary material for: Federated Few-Shot Learning for Mobile NLP
Source: arXiv:2212.05974 source file (2023-08-19)
Supplement: Supplementary file 4 [file sec-appendix-niid.tex]

\subsection{Definition of non-iid}\label{sec:appendix-niid}
\subsubsection{Non-IID. Label Distribution}
\input{fig-def-fsl-distribution}
\input{fig-def-distribution.tex}
We follow the popular FedNLP framework~\cite{lin-etal-2022-fednlp} to use $\alpha$ to define \textbf{Non-IID Label Distributions.}
`12Here we present how we synthesize the data partitions such that clients the share same (or very similar) number of samples, but have different label distributions from each other.
We assume that on every client training, samples are drawn independently with labels following a categorical distribution over L classes parameterized by a vector q (qi $\geq$ 0, i $\in$  [1, L] and $‖q‖$ = 1). 
To synthesize a population of non-identical clients, we draw q $\sim$  DirL($\alpha$p) from a Dirichlet distribution, where p characterizes a prior class distribution over L classes, and $\alpha$ > 0 is a concentration parameter controlling the identicalness among clients. 
For each client $C_{j}$, we draw a $q_{j}$ as its label distribution and then sample samples without replacement from the global dataset according to $q_{j}$. 
With $\alpha$ $\rightarrow$ $\infty$ , all clients have identical distributions to the prior (i.e., uniform distribution); 
with $\alpha$ $\rightarrow$ 0, on the other extreme, each client holds samples from only one class chosen at random. 
As shown in Figure~\ref{fig:def-distribution}, we show a series heatmaps for visualizing the distribution differences between each client.
Figure~\ref{fig:def-gamma} shows an example of the concrete label distributions for all clients with different $\alpha$. 
We can see that when $\alpha$ is smaller, the overall label distribution shift becomes larger.

\subsubsection{Non-IID. Quantity Distribution}
\input{fig-def-fednlp-beta.tex}
It is also common that different clients have very different data quantities while sharing similar label distribution. 
We thus also provide a quantity-level Dirichlet allocation $z$ $\sim$ DirN ($\beta$) where N is the number of clients. 
Then, we can allocate samples in a global dataset to all clients according to the distribution $z$ — i.e., |$D_{i}$| = $z_{i}$|$D_{G}$|. If we would like to model both quantity and label distribution shift, it is also easy to combine both factors. Note that one could assume it is a uniform distribution z $\sim$ U (N ), (or $\beta \rightarrow \infty$ ) if we expect all clients to share similar number of samples. A concrete example is shown in Figure~\ref{fig:def-fednlp-beta} (Appendix).
