# Supplementary material for: Federated Few-Shot Learning for Mobile NLP
Source: arXiv:2212.05974 source file (2023-08-19)
Supplement: Supplementary file 5 [file sec-appendix-overall.tex]

\subsection{Overall Performance}\label{sec:appendix-overall}

\textbf{Gain and Gap}

This section will show two-fold comparison:

1. Show the gain of few shot fedpet (prompting fine-tuning) versus vanilla fedcls (i.e., head fine-tuning)~\cite{scao2021many}.

2. Show the gap from few shot fedpet versus full dataset fine-tuning.

End-to-end exps: convergence plots (line plot. X-axis: clock time; Y-axis: testing accuracy).

\textbf{Accuracy gain turns more obvious when labeled data is extremely few.} Accuracy gain means how much FedPrompt outperforms vanilla fine-tuning, shown in Figure~\ref{fig:eval-performance-gain}.

\input{fig-eval-performance-gain.tex}

\textbf{There is a balance point for each dataset.}
\mwx{Simplify Figure~\ref{fig:eval-performance-overall} to one line. And parallel it with Figure~\ref{fig:eval-performance-gain}}
FedPrompt reaches its best gain when training setting is around the balance point.
Some balance point may be extremely few, e.g., \texttt{AGNEWS}.
While other datasets may need more labeled data to make the sufficient usage of the prompt to the pre-trained models.
Results are shown in Figure~\ref{fig:eval-performance-overall}.

\input{fig-eval-performance-overall.tex}
