# Supplementary material for: Federated Few-Shot Learning for Mobile NLP
Source: arXiv:2212.05974 source file (2023-08-19)
Supplement: Supplementary file 8 [file sec-appendix.tex]

\section*{Appendix} \label{sec:appendix}
\renewcommand\thesubsection{\Alph{subsection}}
\input{sec-appendix-soft-label}

\input{sec-appendix-niid}

\input{sec-appendix-overall.tex}

\input{sec-appendix-models.tex}

\input{sec-appendix-sparsity.tex}

\input{sec-eval-cost.tex}
